# Supplementary material for: PQC Migration of IPsec: Reliable Composite Key Sharing Mechanisms in IKEv2
Source: arXiv:2610.25799 source file (2026-10-19)
Supplement: Supplementary file 1 [file 10_appendix_artifact.tex]

\section*{ARTIFACT APPENDIX}
A major goal of our research is the creation of reproducible experiments and the publication of associated measurement data. 
